# Supplementary material for: Effect of $R$-site substitution and the pressure on stability of $R$Fe$_{12}$: A first-principles study
Source: arXiv:1805.12241 ancillary file (2018-09-25)
Supplement: Supplementary file 1 [file suppl_zrstr.pdf]

# Supplemental Material to "Effect of $R$-site substitution and pressure on stability of $R\mathrm{Fe}_{12}$: A first-principles study"

Yosuke Harashima,[1,3] Taro Fukazawa,[1,3] Hiori Kino,[2,3] and Takashi Miyake[1,2,3]
[1)] *Research Center for Computational Design of Advanced Functional Materials, National Institute of Advanced Industrial Science and Technology, Tsukuba, Ibaraki 305-8568, Japan*
[2)] *Center for Materials Research by Information Integration, MaDIS, National Institute for Materials Science, Tsukuba, Ibaraki 305-0047, Japan*
[3)] *Elements Strategy Initiative Center for Magnetic Materials, National Institute for Materials Science, Tsukuba, Ibaraki 305-0047, Japan*

(Dated: 6 September 2018)

In this material, we present the following information.

**SA:** Lattice constants of $R\mathrm{Fe}_{12}$ and $R_2\mathrm{Fe}_{17}$.

**SB:** Calculated atomic radii of $R$ and Fe.

**SC:** Difference of the total energy between the rhombohedral and the hexagonal $R_2\mathrm{Fe}_{17}$.

**SD:** Bond lengths in $R\mathrm{Fe}_{12}$.

**SE:** Lattice distortion in $\mathrm{NdFe}_{12}$ and $\mathrm{Nd}_2\mathrm{Fe}_{17}$ induced by hydrostatic pressure.

## SA. Lattice constants of $R\mathrm{Fe}_{12}$ and $R_2\mathrm{Fe}_{17}$

TABLE SI. The lattice constants of $R\mathrm{Fe}_{12}$ with the $\mathrm{ThMn}_{12}$ structure in the unit of Å, where $R$=La, Pr, Nd, Sm, Gd, Dy, Ho, Er, Tm, Lu, Y, Sc, Zr, Hf are considered. The space group is $I4/mmm$, No. 139. The $R\mathrm{Fe}_{12}$ consists of $R(2a)$, Fe($8f$), Fe($8i$) and Fe($8j$). An $R(2a)$-site is at (0, 0, 0); an Fe($8f$)-site is at (0.25, 0.25, 0.25); an Fe($8i$)-site is at ($x_{8i}$, 0, 0); an Fe($8j$)-site is at ($x_{8j}$, 0.5, 0). The inner coordinates $x_{8i}$ for Fe($8i$) and $x_{8j}$ for Fe($8j$) are shown in this table.

| | La | Pr | Nd | Sm | Gd | Dy | Ho | Er | Tm | Lu | Y | Sc | Zr | Hf |
|---|---|---|---|---|---|---|---|---|---|---|---|---|---|---|
| $a$ | 8.592 | 8.554 | 8.533 | 8.497 | 8.467 | 8.442 | 8.431 | 8.421 | 8.412 | 8.395 | 8.453 | 8.347 | 8.330 | 8.309 |
| $c$ | 4.675 | 4.679 | 4.681 | 4.687 | 4.691 | 4.689 | 4.688 | 4.687 | 4.686 | 4.684 | 4.691 | 4.674 | 4.659 | 4.654 |
| $x_{8i}$ | 0.3603 | 0.3597 | 0.3594 | 0.3588 | 0.3584 | 0.3581 | 0.3580 | 0.3578 | 0.3577 | 0.3575 | 0.3583 | 0.3568 | 0.3575 | 0.3573 |
| $x_{8j}$ | 0.2650 | 0.2666 | 0.2676 | 0.2696 | 0.2714 | 0.2729 | 0.2735 | 0.2741 | 0.2747 | 0.2758 | 0.2721 | 0.2793 | 0.2780 | 0.2792 |

TABLE SII. The lattice constants of $R_2\mathrm{Fe}_{17}$ with the rhombohedral $\mathrm{Th}_2\mathrm{Zn}_{17}$-type structure in the unit of Å, where $R$=La, Pr, Nd, Sm, Gd, Dy, Ho, Er, Tm, Lu, Y, Sc, Zr, Hf are considered. The space group is $R\bar{3}m$, No. 166. The rhombohedral $R_2\mathrm{Fe}_{17}$ consists of the $R$(6c), Fe($18f$), Fe($18h$), Fe($9d$) and Fe($6c$) atoms. An $R(6c)$-site is at (0, 0, $z_{R6c}$); an Fe($18f$)-site is at ($x_{18f}$, 0, 0); an Fe($18h$)-site is at ($x_{18h}$, $-x_{18h}$, $z_{18h}$); an Fe($9d$)-site is at (0.5, 0, 0.5); an Fe($6c$)-site is at (0, 0, $z_{\mathrm{Fe6c}}$). These inner coordinates, $z_{R6c}$, $x_{18f}$, $x_{18h}$, $z_{18h}$ and $z_{\mathrm{Fe6c}}$, are shown in this table.

| | La | Pr | Nd | Sm | Gd | Dy | Ho | Er | Tm | Lu | Y | Sc | Zr | Hf |
|---|---|---|---|---|---|---|---|---|---|---|---|---|---|---|
| $a$ | 8.599 | 8.580 | 8.562 | 8.526 | 8.491 | 8.413 | 8.391 | 8.376 | 8.361 | 8.335 | 8.455 | 8.241 | 8.231 | 8.200 |
| $c$ | 12.613 | 12.519 | 12.489 | 12.455 | 12.438 | 12.409 | 12.393 | 12.380 | 12.369 | 12.354 | 12.410 | 12.372 | 12.427 | 12.415 |
| $z_{R6c}$ | 0.3412 | 0.3410 | 0.3410 | 0.3407 | 0.3405 | 0.3404 | 0.3404 | 0.3402 | 0.3401 | 0.3398 | 0.3408 | 0.3385 | 0.3403 | 0.3399 |
| $x_{18f}$ | 0.2864 | 0.2892 | 0.2905 | 0.2927 | 0.2946 | 0.2994 | 0.3009 | 0.3021 | 0.3031 | 0.3048 | 0.2964 | 0.3107 | 0.3106 | 0.3117 |
| $x_{18h}$ | 0.5021 | 0.5014 | 0.5011 | 0.5006 | 0.5002 | 0.4999 | 0.4998 | 0.4997 | 0.4995 | 0.4993 | 0.5000 | 0.4985 | 0.4988 | 0.4984 |
| $z_{18h}$ | 0.1578 | 0.1575 | 0.1573 | 0.1571 | 0.1572 | 0.1584 | 0.1587 | 0.1588 | 0.1589 | 0.1590 | 0.1578 | 0.1594 | 0.1592 | 0.1592 |
| $z_{\mathrm{Fe6c}}$ | 0.0958 | 0.0962 | 0.0964 | 0.0965 | 0.0964 | 0.0958 | 0.0957 | 0.0956 | 0.0956 | 0.0955 | 0.0962 | 0.0953 | 0.0952 | 0.0950 |

Table SI shows the computationally optimized lattice constants of $R\mathrm{Fe}_{12}$ ($R$ = La, Pr, Nd, Sm, Gd, Dy, Ho, Er, Tm, Lu, Y, Sc, Zr, Hf). Table SII and Table SIII show the lattice constants of $R_2\mathrm{Fe}_{17}$ with the (rhombohedral) $\mathrm{Th_2Zn_{17}}$ structure and those with the (hexagonal) $\mathrm{Th_2Ni_{17}}$ structure, respectively. The inner coordinates determined by the computational structure optimization are also shown in the tables.

TABLE SIII. The lattice constants of $R_2\mathrm{Fe}_{17}$ with the hexagonal $\mathrm{Th_2Ni_{17}}$-type structure in the unit of Å, where $R$=La, Pr, Nd, Sm, Gd, Dy, Ho, Er, Tm, Lu, Y, Sc, Zr, Hf are considered. The space group is $P6_3/mmc$, No. 194. the hexagonal $R_2\mathrm{Fe}_{17}$ consists of the $R(2b)$, $R(2d)$, Fe($12j$), Fe($12k$), Fe($6g$) and Fe($4f$) atoms. An $R(2b)$-site is at (0, 0, 0.25); an $R(2d)$-site is at (2/3, 1/3, 0.25); an Fe($12j$)-site is at ($x_{12j}$, $y_{12j}$, 0.25); an Fe($12k$)-site is at ($x_{12k}$, $2x_{12k}$, $z_{12k}$); an Fe($6g$)-site is at (0.5, 0, 0); an Fe($4f$)-site is at (1/3, 2/3, $z_{4f}$). These inner coordinates, $x_{12j}$, $y_{12j}$, $x_{12k}$, $z_{12k}$ and $z_{4f}$, are shown in this table.

| | La | Pr | Nd | Sm | Gd | Dy | Ho | Er | Tm | Lu | Y | Sc | Zr | Hf |
|---|---|---|---|---|---|---|---|---|---|---|---|---|---|---|
| $a$ | 8.591 | 8.580 | 8.562 | 8.531 | 8.492 | 8.420 | 8.375 | 8.357 | 8.341 | 8.312 | 8.463 | 8.233 | 8.229 | 8.209 |
| $c$ | 8.409 | 8.334 | 8.313 | 8.282 | 8.269 | 8.272 | 8.284 | 8.280 | 8.276 | 8.271 | 8.261 | 8.261 | 8.295 | 8.279 |
| $x_{12j}$ | 0.3300 | 0.3297 | 0.3296 | 0.3293 | 0.3292 | 0.3295 | 0.3296 | 0.3295 | 0.3293 | 0.3292 | 0.3293 | 0.3289 | 0.3292 | 0.3290 |
| $y_{12j}$ | 0.9519 | 0.9537 | 0.9551 | 0.9572 | 0.9595 | 0.9633 | 0.9653 | 0.9662 | 0.9671 | 0.9687 | 0.9609 | 0.9743 | 0.9745 | 0.9756 |
| $x_{12k}$ | 0.1673 | 0.1667 | 0.1665 | 0.1663 | 0.1661 | 0.1658 | 0.1657 | 0.1656 | 0.1656 | 0.1654 | 0.1660 | 0.1649 | 0.1647 | 0.1645 |
| $z_{12k}$ | 0.9875 | 0.9861 | 0.9856 | 0.9848 | 0.9851 | 0.9864 | 0.9871 | 0.9870 | 0.9869 | 0.9869 | 0.9857 | 0.9871 | 0.9877 | 0.9873 |
| $z_{4f}$ | 0.1075 | 0.1069 | 0.1068 | 0.1065 | 0.1065 | 0.1069 | 0.1074 | 0.1075 | 0.1075 | 0.1076 | 0.1068 | 0.1077 | 0.1075 | 0.1075 |

## SB. Calculated atomic radii of $R$ and Fe

TABLE SIV. The calculated atomic radii $r_R^{\mathrm{calc}}$ and $r_{\mathrm{Fe}}^{\mathrm{calc}}$ in the unit of Å, where $R$=La, Pr, Nd, Sm, Gd, Dy, Ho, Er, Tm, Lu, Y, Sc, Zr, Hf. The structures are also shown.

| | La | Pr | Nd | Sm | Gd | Dy | Ho | Er | Tm | Lu | Y | Sc | Zr | Hf | Fe |
|---|---|---|---|---|---|---|---|---|---|---|---|---|---|---|---|
| | dhcp | dhcp | dhcp | dhcp | hcp | hcp | hcp | hcp | hcp | hcp | hcp | hcp | hcp | hcp | bcc |
| $r_{R,\mathrm{Fe}}^{\mathrm{calc}}$ | 1.858 | 1.838 | 1.823 | 1.801 | 1.779 | 1.756 | 1.746 | 1.736 | 1.730 | 1.691 | 1.767 | 1.606 | 1.595 | 1.572 | 1.228 |

Table SIV shows the calculated values of the atomic radii for $R$ and Fe. Those values are a half of the nearest neighbor distance in the simple substances (the dhcp structure is assumed for $R$=La, Pr, Nd, Sm; the hcp structure is assumed for $R$=Gd, Dy, Ho, Er, Tm, Lu, Y, Sc, Zr, Hf; the bcc structure is assumed for Fe).

## SC. Energy difference between rhombohedral and hexagonal $R_2$Fe$_{17}$

Figure S1 shows difference of the total energy between $R_2\mathrm{Fe}_{17}$ with the (rhombohedral) $\mathrm{Th_2Zn_{17}}$ structure and that with the (hexagonal) $\mathrm{Th_2Ni_{17}}$ structure. The energy difference is defined as,

$$\Delta E \,|^{\frac{1}{2}R_2\mathrm{Fe}_{17}(\mathrm{rmb})\leftarrow\frac{1}{2}R_2\mathrm{Fe}_{17}(\mathrm{hex})} \equiv \frac{1}{2}\left(E[R_2\mathrm{Fe}_{17}(\mathrm{rmb})] - E[R_2\mathrm{Fe}_{17}(\mathrm{hex})]\right), \tag{S1}$$

where $R_2\mathrm{Fe}_{17}$(rmb) and $R_2\mathrm{Fe}_{17}$(hex) denote $R_2\mathrm{Fe}_{17}$ with the $\mathrm{Th_2Zn_{17}}$ and $\mathrm{Th_2Ni_{17}}$ structures, respectively. It does not reproduce very well the experimental observation that the $\mathrm{Th_2Zn_{17}}$ structure is found with light rare-earth elements, while the $\mathrm{Th_2Ni_{17}}$ structure is found with heavy rare-earth elements (see e.g. Ref. 1). However, the tendency of the heavy lanthanoids to prefer the $\mathrm{Th_2Ni_{17}}$ structure can be seen in the figure: the $\mathrm{Th_2Ni_{17}}$ structure becomes more stable against the $\mathrm{Th_2Zn_{17}}$ structure as $r_R^{\mathrm{calc}}$ decreases.

## SD. Bond lengths in $R$Fe$_{12}$

In this section, we analyze local structure around an $R$ atom in $R\mathrm{Fe}_{12}$, which is closely related to the anisotropic behavior in the lattice constants (Fig. 3). We focus on the atomic bonds $R(2a)$–Fe($8i$), $R(2a)$–Fe($8j$), and Fe($8j$)–

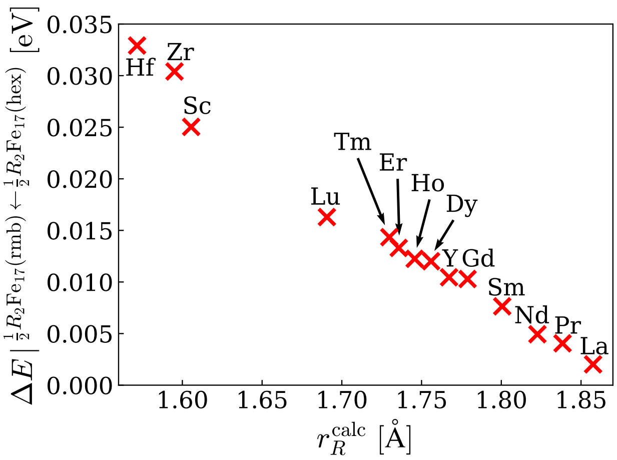


FIG. S1. (Color online) The energy difference defined by Eq. (S1) for $R$=La, Pr, Nd, Sm, Gd, Dy, Ho, Er, Tm, Lu, Y, Sc, Zr, Hf as a function of the atomic radius $r_R^{\mathrm{calc}}$.

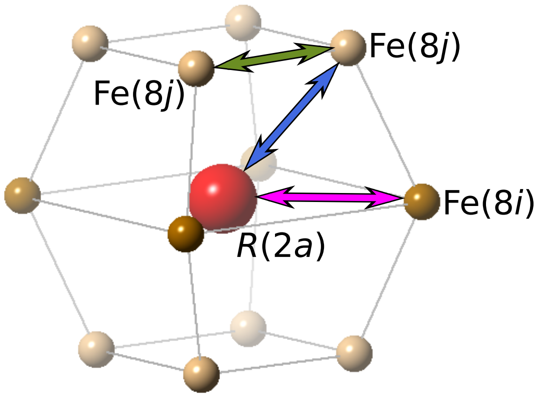


FIG. S2. (Color online) Local structure surrounding an $R$ atom in $R\mathrm{Fe}_{12}$. The pairs of $R(2a)$–Fe$(8i)$, $R(2a)$–Fe$(8j)$ and Fe$(8j)$–Fe$(8j)$ that we plot their $r_R^{\mathrm{calc}}$ dependence in Fig. S3 are denoted by arrows.

Fe$(8j)$, which is illustrated in Fig. S2. Note that the inner coordinates can be determined from the length of the bonds.

The left panel in Fig. S3 shows the length of the two $R$–Fe bonds, $r_{2a-8i}$ of $R(2a)$–Fe$(8i)$ and $r_{2a-8j}$ of $R(2a)$–Fe$(8j)$, as functions of $r_R^{\mathrm{calc}}$. $r_{2a-8i}$ and $r_{2a-8j}$ are almost identical to each other for all the cases. The sum of the atomic radii of $R$ and Fe, $r_R^{\mathrm{calc}} + r_{\mathrm{Fe}}^{\mathrm{calc}}$ (see also Table SIV), which can be interpreted as a typical length between $R$ and Fe, are also plotted. Comparing the bond-lengths with the sum of the atomic radii, the deviation systematically increases as $r_R^{\mathrm{calc}}$ decreases.

The right panel in Fig. S3 shows the bond-length, $r_{8j-8j}$ of the nearest Fe$(8j)$–Fe$(8j)$ pair in $R\mathrm{Fe}_{12}$. As $r_R^{\mathrm{calc}}$ decreases, the value of $r_{8j-8j}$ approaches the sum of the atomic radii, $2r_{\mathrm{Fe}}^{\mathrm{calc}}$, which is considered as a typical length between Fe atoms. This is opposite to the trend in the two $R$–Fe bonds.

### SE. Lattice distortion under pressure

The left panel in Fig. S4 shows values of $a(p)/a(0)$ and $c(p)/c(0)$ of $\mathrm{NdFe}_{12}$ where $a(p)$ and $c(p)$ denote the lattice constant $a$ and $c$ under hydrostatic pressure $p$; the right panel in the figure shows $a(p)/a(0)$ and $c(p)/c(0)$ of $\mathrm{Nd_2Fe_{17}}$. In both systems, the ratio for $a$ is smaller than the ratio for $c$ except for the one at the highest pressure in $\mathrm{Nd_2Fe_{17}}$. The tendency of $a$ to be more susceptible than $c$ was seen also in their dependence on the atomic radius of $R$, which is shown in Fig. 3.

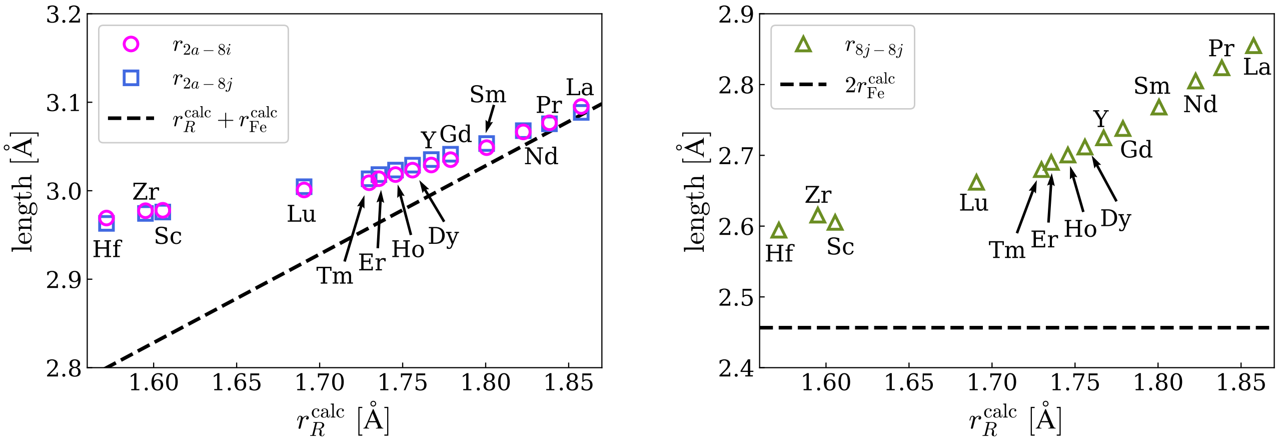


FIG. S3. (Color online) The lengths of the $R(2a)$–Fe($8i$), $R(2a)$–Fe($8j$), and Fe($8j$)–Fe($8j$) bond that are depicted in Fig. S2 calculated for $R$=La, Pr, Nd, Sm, Gd, Dy, Ho, Er, Tm, Lu, Y, Sc, Zr, Hf. They are referred to as $r_{2a-8i}$ and $r_{2a-8j}$ in the left panel, and $r_{8j-8j}$, in the right panel, respectively. In the left panel, the sum of $r_R^{calc}$ and $r_{Fe}^{calc}$ is plotted as a line; in the right panel the value of $2r_{Fe}^{calc}$ is plotted as a horizontal line.

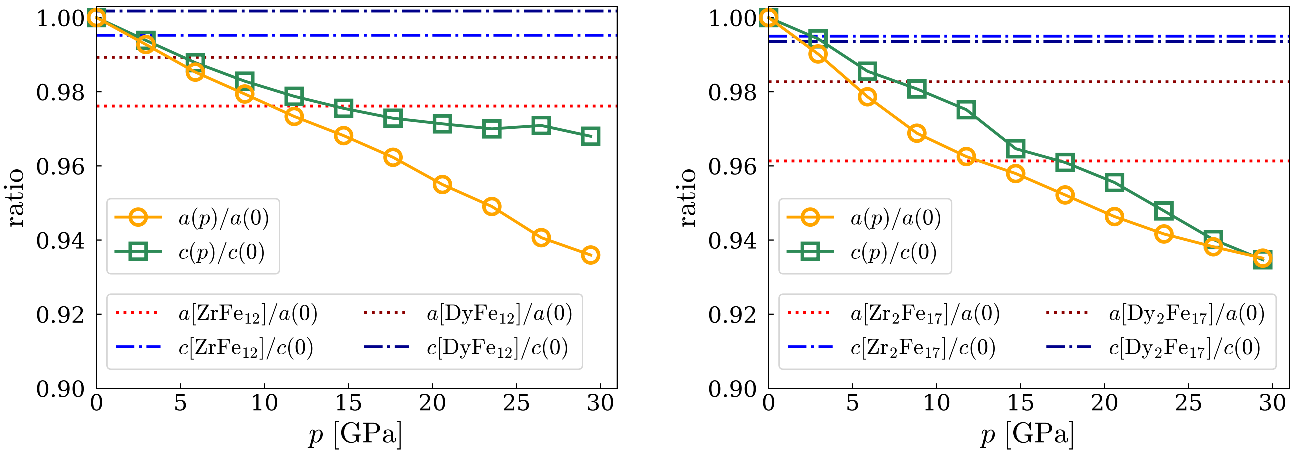


FIG. S4. (Color online) Ratio of the lattice constants $a(p)/a(0)$ and $c(p)/c(0)$ of $NdFe_{12}$ (left panel) and $Nd_2Fe_{17}$ (right panel) under hydrostatic pressure $p$. The horizontal lines in the left panel show the ratio of $a$ for $ZrFe_{12}$ and $DyFe_{12}$ to that for $NdFe_{12}$ ($a[ZrFe_{12}]/a(0)$ and $a[DyFe_{12}]/a(0)$), and the ratio of $c$ for $ZrFe_{12}$ and $DyFe_{12}$ to that for $NdFe_{12}$ ($c[ZrFe_{12}]/c(0)$ and $c[DyFe_{12}]/c(0)$) at zero pressure; the horizontal lines in the right panel show the ratio of $a$ for $Zr_2Fe_{17}$ and $Dy_2Fe_{17}$ to that for $Nd_2Fe_{17}$ ($a[Zr_2Fe_{17}]/a(0)$ and $a[Dy_2Fe_{17}]/a(0)$), and the ratio of $c$ for $Zr_2Fe_{17}$ and $Dy_2Fe_{17}$ to that for $Nd_2Fe_{17}$ ($c[Zr_2Fe_{17}]/c(0)$ and $c[Dy_2Fe_{17}]/c(0)$) at zero pressure.

[1]K. Koyama and H. Fujii, Phys. Rev. B **61**, 9475 (2000).
